# Supplementary material for: Learning Complementary Agent Groups via Task Hypergraphs for Next-POI Recommendation with Missing Modalities
Source: arXiv:2610.25801 source file (2026-10-19)
Supplement: Supplementary file 1 [file 09_appendix.tex]

\section{Agent Interfaces and Execution Details}
\label{app:roles}
The six agents analyze long-term preference, recent trajectories, time and distance, available text, available images, and permitted collaborative histories. Legal operation parameters are generated deterministically from the task: history segments, retrieval ranges, or candidate pairs. Retrieval queries use available task, candidate, and admitted message states.

An operation by agent $a$ in task hyperedge $e$ returns
\begin{equation}
O_{a,e}=\bigl(\{m_{a,e,p}\}_{p\in T_e},d_{a,e},\mathcal I_{a,e},\sigma_{a,e},c_{a,e}\bigr),
\end{equation}
where $T_e$ is the target set, $m_{a,e,p}$ a candidate message, $d_{a,e}$ a task summary, $\mathcal I_{a,e}$ the accessed objects and coverage, $\sigma_{a,e}$ execution status, and $c_{a,e}$ measured cost. Empty results and cache hits are explicit. Candidate messages are vectors, not independently calibrated scores. The trajectory agent may retrieve related visit sequences; the collaborative retrieval agent may search other users or related POIs. Data access, task relevance, and budget restrict these operations.

The executor uses a shared frozen LLM, role-specific LoRA adapters, and trainable input/output projections. Available text enters as tokens; encoded images and trajectories enter through continuous projections. Hidden states at candidate readout positions are projected to $m_{a,e,p}$; a separate position provides the summary. Ranking gradients pass through continuous execution while discrete retrieval choices condition the retrieved inputs.

Request-level agent memory summarizes completed work; task-local agent state belongs to one task. Only participating agent memories and target candidates are updated. Nonmembers cannot read detailed task messages. Candidates outside the task target set $T_e$ retain their previous ranking states $v_p^{(t)}$ without modification; within $T_e$, any uncovered candidate retains its previous task result $z_{e,p}$, and repeated messages replace rather than duplicate contributions. Missing target images remain missing when historical images inform visual preference. No raw-modality reconstruction head is used; spatiotemporal analysis uses known distances and historical transitions, not unavailable future dwell or travel-time labels.

\section{Inference Procedure}
\label{app:algorithm}
\begin{enumerate}
\item Initialize request/candidate states, agent memories, base scores, masks, and the budget ledger from legal pre-prediction inputs.
\item Select a task, targets, and initiator, or STOP. Invite eligible members conditioned on the selected set until EXECUTE; reserve the required costs.
\item Initialize a fixed-membership task hyperedge. Each round selects operations and legal parameters from a common snapshot, reserves joint costs, executes admitted operations, and retains the latest agent--target messages.
\item Aggregate covered messages, preserve empty states, broadcast results, and update local states. Repeat while legal work and local limits permit.
\item Update participating memories and target candidates, and the request state for a request-state-update task. Recompute all scores with Equation~\ref{eq:rank}, reconcile reservations once, and return to step 2 until stopping or a global limit.
\end{enumerate}
\section{Training Records and Evaluation Conventions}
\label{app:repro}
Training records retain the request cutoff, masks, fixed pool, base scores, task, targets, initiator, invitation order, legal masks, operation parameters, retrieval scope, coverage, statuses, and costs. PPO additionally retains old conditional probabilities, critic values, and rewards. Labels are evaluated outside the policy and tool interfaces. Simultaneous member decisions share the same round-start observation. Combination records use training requests only; after executor updates, both combination evaluation and PPO trajectories are refreshed.

\paragraph{Warm-up supervision.}
Execution parameters $\phi$ include input projections, role adapters, and hidden-state readout projections. Parameters $\psi$ include message encoders, gated updates, and the ranking head. Ranking supervision applies at completed task states and may average multiple stopping positions. Retrieved objects are conditional inputs, while the action trajectory is fixed. The set evaluator $Q_\omega$ uses measured outcomes of executed combinations under the recorded conditions; it does not label unexecuted combinations or estimate intrinsic group ability. Single-task utility does not by itself determine global stopping.

\paragraph{Initial state and repeated processing.}
At initialization, identical correction terms in Equation~\ref{eq:rank} cancel in value and derivative. Both use the same deterministic scoring function, with the initial reference retained in the warm-up computation graph. No-collaboration records supervise stopping but provide zero executor gradient. Executed no-new-content records can change recurrent states and receive ranking gradients; recurrence is not assumed idempotent.

\paragraph{Rewards and termination.}
The final discrete transition of task $t$ receives $U_{t+1}-U_t-\lambda_{\mathrm{cost}}c_t$ once; intermediate transitions receive zero. Sampled global STOP incurs only its decision cost. Forced termination adds no fictitious STOP or duplicate charge. GAE uses $\gamma=1$, $\lambda_{\mathrm{GAE}}=0.95$. Across 1,000 sampled rollout episodes, the cumulative reward matches the telescoping return $\sum_{t=0}^{T-1} R_t - (U_T - U_0 - \lambda_{\mathrm{cost}}\sum_{t=0}^{T-1}c_t)$ within floating-point tolerance ($<10^{-7}$ numerical discrepancy under float32 summation).

\paragraph{Synchronous budgets.}
Round-start operations reserve their joint upper-bound costs plus routing and aggregation. Admission proceeds in ascending estimated cost, with observations held fixed; masks and admissions are retained for PPO. Text generation is capped at 128 tokens. Unused reservations are returned. No affordable operation causes forced termination without a sampled STOP. Matched controls use the same reservations and caps.

\paragraph{Metric denominators.}
Coverage is the fraction of requests whose target is in the fixed pool. Conditional scores average covered requests; end-to-end scores average all requests with zero for retrieval misses. Under request-macro weighting, end-to-end score equals coverage times conditional score. For one relevant target, Recall@$L$ equals Hit@$L$; reciprocal rank is zero on misses. User-macro weighting is labeled separately.

\subsection{Policy objective and training extensions}
\label{app:policy}
For each discrete decision $i$, PPO records the permitted observation $o_i$, sampled action $a_i$, legal mask, old conditional probability, value estimate, and subsequent rewards. The policy maximizes
\begin{equation}
\mathcal J_{\mathrm{clip}}(\theta)=\mathbb E_i\!\left[
\min\!\left(\rho_i(\theta)\widehat A_i,
\operatorname{clip}(\rho_i(\theta),1-\epsilon,1+\epsilon)\widehat A_i\right)\right],
\label{eq:ppo}
\end{equation}
where $\rho_i(\theta)=\pi_\theta(a_i\mid o_i)/\pi_{\theta_{\mathrm{old}}}(a_i\mid o_i)$ and $\widehat A_i$ is the advantage estimate. The shared critic has parameters $\eta$. The same legal mask is retained when recomputing sampled action probabilities; tool execution parameters are deterministically bound to task targets and legal ranges without stochastic parameter sampling, and forced actions are excluded as learned choices. Invitations and local decisions receive later rewards through advantage estimation, without artificial per-agent complementarity bonuses.

Summing Equation~\ref{eq:return} over a finite undiscounted episode gives
\begin{equation}
\sum_{t=0}^{T-1}R_t=U_T-U_0-\lambda_{\mathrm{cost}}\sum_{t=0}^{T-1}c_t.
\label{eq:telescope}
\end{equation}
Here $T$ counts task and terminal transitions. Successive utilities cancel, and each cost is charged once. The log-probability utility is distinct from NDCG; ranking metrics determine evaluation and validation model selection.

An optional extension alternates executor updates under a frozen policy with PPO on newly collected trajectories when the policy shifts the executor's input distribution. Executor changes require refreshing combination outcomes and policy data. The primary design uses frozen execution modules during PPO.
