# Supplementary material for: Learning Complementary Agent Groups via Task Hypergraphs for Next-POI Recommendation with Missing Modalities
Source: arXiv:2610.25801 source file (2026-10-19)
Supplement: Supplementary file 2 [file 09_appendix_extended.tex]

\section{Agent Interfaces and Execution Details}
\label{app:roles}
Table~\ref{tab:roles} specifies the six processing roles. Each execution also reports object identifiers, coverage, operation status, and actual cost. A role can send an existing result, update its assessment using the shared task state, or finish. The executor input includes candidate indices, role identifiers, operation identifiers, missingness markers, and task descriptions. Explanatory text is optional output for inspection; candidate vectors provide the ranking interface.

\begin{table*}[t]
\centering\small
\caption{Capability interfaces in the proposed executor. The listed choices are legal operations, not mandatory calls on every request.}
\label{tab:roles}
\begin{tabular}{@{}>{\raggedright\arraybackslash}p{0.16\linewidth}>{\raggedright\arraybackslash}p{0.24\linewidth}>{\raggedright\arraybackslash}p{0.30\linewidth}>{\raggedright\arraybackslash}p{0.20\linewidth}@{}}
\toprule
Role & Accessible input & Example operation choices & Candidate output \\
\midrule
Long-term preference & Pre-prediction history and available content & Read a behavior summary; select task-relevant history; compare history and candidates using group results & Preference matching \\
Short-term trajectory & Recent order, categories, legal time gaps & Analyze activity sequence; retrieve similar segments; reconsider transitions using messages & Trajectory matching \\
Spatiotemporal analysis & Known location and time, distances, historical transitions & Compare distances and observed transitions; revise target comparisons & Spatial/temporal matching \\
Text analysis & Available descriptions and reviews & Retrieve relevant passages; extract POI attributes; compare target POIs & Text attributes and matching \\
Visual analysis & Available candidate or historical images & Analyze target images; select relevant historical images; compare visual features & Visual preference or candidate features \\
Collaborative retrieval & Permitted training histories and POI indices & Retrieve similar users, trajectories, or related POIs; revise query from shared results & Retrieved identifiers and matching \\
\bottomrule
\end{tabular}
\end{table*}

\paragraph{Legal operations and query construction.}
The policy first selects an operation type and then a legal parameter, such as a target history segment, retrieval range, or candidate pair. Deterministic rules generate the parameter choices from the task. Retrieval queries use the available task, candidate, and received-message states, with a specified index scope and ranking rule. Empty results and cache hits are represented explicitly. Short-term sequence retrieval and collaborative retrieval can share an index, but their query conditions and returned objects remain distinguishable.

\paragraph{State isolation and coverage.}
The request-level memory $h_a^{(t)}$ summarizes a role's completed work; $l_{a,e}$ belongs only to the current task. Completing an edge updates its participating memories and target candidate states, while its summary remains an independent task record. Nonparticipating roles do not implicitly read its detailed messages. A coverage mask excludes unprocessed candidates from message aggregation. When no valid member covers a candidate, Equation~\ref{eq:edge} preserves its task state. Retransmitting or caching a message does not create a new member contribution. Gated state transitions can still react to repeated processing, which motivates the no-new-content diagnostic in Section~\ref{sec:evaluation}.

\paragraph{Observed and inferred semantics.}
Semantic compensation can use available text, collaborative retrieval, or historical images to improve a candidate representation. A missing target image remains missing, even when historical images inform visual preference. If no relevant images exist, visual analysis is masked out. Without travel-time or future-dwell information, the spatiotemporal role analyzes distances and historical transitions rather than supplying travel-feasibility labels. The primary design includes no raw-modality reconstruction head. An auxiliary embedding-reconstruction target is a possible separate comparison only where artificially masked training examples supply legal ground truth.

\section{Inference Procedure}
\label{app:algorithm}
The pseudocode describes the specified episode, including the option to return the base ranking. All loops have configured finite execution limits. Operation reservations include necessary execution costs; any selection cost is logged even if the policy stops. Configuration values are determined through implementation and validation, not fixed by this algorithm.

\begin{center}
\fbox{\begin{minipage}{0.94\linewidth}
\textbf{Algorithm 1: Request-level task-hypergraph reranking}\\[3pt]
\textbf{Input:} legal history, time, and location, fixed candidates, observed content and masks, budget.\\
\textbf{Initialize:} base scores, request/candidate states, request-level memories, empty task hypergraph.
\begin{enumerate}
\item While budget and execution limits permit:
\begin{enumerate}
\item Generate executable task--target pairs from the current ranking and masks. Select STOP or a pair; charge the selection cost. If STOP, finish.
\item Select a legal initiator, charge its routing cost, and initialize the member set.
\item Until EXECUTE or no further invitation is legal, encode the current member set, select a new member or EXECUTE, and charge routing cost. Add only unselected legal members.
\item Create the task hyperedge and initialize shared and member-local states. Keep membership fixed during this task.
\item While legal member work remains and local limits permit:
\begin{enumerate}
\item From the round-start snapshot, select member operations and legal parameters; reserve their joint execution cost within the remaining budget.
\item Execute selected operations; return messages, coverage, statuses, and actual cost. Retain the latest role--target message.
\item Aggregate only covered selected-member messages. Preserve empty candidate states. Broadcast task results and update local states.
\end{enumerate}
\item Update participating memories and target candidate states. Update request state if the task is a request-state update.
\item Recompute all candidate scores using Equation~\ref{eq:rank}; reconcile reservations with actual costs, without charging logged routing costs again.
\end{enumerate}
\item Return the current ranking and execution records.
\end{enumerate}
\end{minipage}}
\end{center}

\paragraph{Illustrative execution.}
For a request containing an image-missing coffee shop, a request-state-update task might first select trajectory and preference capabilities. After those members analyze legal history and exchange results, the ranking head reads the updated states. A later comparison task could reuse preference and invite text analysis for two coffee shops. A visual member would be legal only if relevant images remain available, for example in the user's history. The same preference role retains distinct task-local states and transfers only the completed-task summary through its request-level memory. This example specifies possible data flow; it supplies neither a fixed team template nor a measured ranking improvement.

\section{Training Records and Evaluation Conventions}
\label{app:repro}
\begin{table*}[t]
\centering\small
\caption{Parameter ownership in the primary training schedule.}
\label{tab:parameters}
\begin{tabular}{p{0.15\linewidth}p{0.48\linewidth}p{0.27\linewidth}}
\toprule
Parameters & Modules & Update source \\
\midrule
Fixed & Base recommender and retrieval, content encoders, LLM base weights & Fixed after base preparation \\
$\phi$ & Executor input projections, role adapters, candidate and task-summary readouts & Supervised ranking loss \\
$\psi$ & Message aggregation, gated states, shared ranking head & Supervised ranking loss \\
$\theta$ & Task, initiator, invitation, local-action, stopping heads and policy state encoder & Behavior warm-up, then PPO \\
$\eta$ & Shared critic & Sampled team returns \\
$\omega$ & Complete-member-set utility evaluator & Executed training combinations; warm-up only \\
\bottomrule
\end{tabular}
\end{table*}

\paragraph{Logging the decision process.}
The training-record schema includes a request identifier and prediction cutoff, masks, candidate pool and base scores, task and target, initiator, invitation order, legal masks, operation parameters, tool scope, coverage, statuses, and costs. Policy records additionally retain old conditional action probabilities, critic values, and rewards. The evaluator computes labels and utility outside the decision interface. Synchronous member decisions store their shared round-start observation; arbitrary serialization of those decisions must not change what members can observe. Subsequent advantages include later task rewards, so an invitation without immediate utility can still receive credit for useful downstream execution.

\paragraph{Warm-up data and changes of executor.}
Combination outcomes are comparable only under recorded execution conditions. Stochastic execution requires repeated records or averaged estimates with their variability retained. Training-only records from earlier combination studies can be reused if the data partitions and execution conditions match. Validation and test outcomes do not become training records. If the executor changes, old combination outcomes no longer describe that executor, and PPO requires fresh trajectories. Optional alternating training retains some random legal tasks and groups to reduce concentration on the current policy's preferred combinations.

\paragraph{Metric denominators.}
Let $\mathcal Q$ be evaluated requests and $\mathcal Q_{\mathrm{cov}}=\{q\in\mathcal Q:p_q^+\in\C_q\}$. Coverage is $|\mathcal Q_{\mathrm{cov}}|/|\mathcal Q|$. For a single next-POI target, let $k_q$ be its rank when covered and $k_q=\infty$ otherwise. A cutoff $L$ gives per-request Hit@$L$ as $\mathbf1[k_q\le L]$ and NDCG@$L$ as $\mathbf1[k_q\le L]/\log_2(k_q+1)$ for finite $k_q$, with zero for misses. Reciprocal rank is $1/k_q$ for finite $k_q$ and zero for misses; any cutoff must be declared. With one relevant target, request-level Recall@$L$ equals Hit@$L$. Conditional metrics average over $\mathcal Q_{\mathrm{cov}}$, while end-to-end metrics average over $\mathcal Q$. The primary aggregation is request-macro; user-macro aggregation assigns different weights and is labeled separately for supplementary results.

\paragraph{Configuration and reporting.}
Appendix~\ref{app:exp} records data processing, baseline adaptations, hyperparameters, and measurement definitions. Table~\ref{tab:config} records executed methodological choices and hyperparameters across all training phases.

\paragraph{Initial-state loss and repeated processing.}
At initialization, the two correction terms in Equation~\ref{eq:rank} have identical arguments. Their values and derivatives cancel, so $\nabla_{\phi,\psi}\mathcal L_{\mathrm{rank}}(S_0)=0$ when the base recommender is fixed. No-collaboration records provide a reference utility and can supervise policy stopping through executed returns; they do not train the executor to avoid unnecessary work. Executed no-new-content trajectories are different: recurrent state updates can change the scores and receive ranking gradients even when no additional objects are retrieved. Their inclusion and the repeated-task diagnostic test this behavior without assuming that state recurrence is idempotent. Both correction evaluations must use the same deterministic scoring function; unmatched stochastic dropout would invalidate exact initial cancellation. The initial reference remains in the computation graph during ranking warm-up, rather than being detached or reused across parameter updates.

\paragraph{Reward placement and episode boundaries.}
Discrete decisions within a task receive zero immediate reward until the task's utility change and total cost are evaluated. We record this reward once, on the final decision preceding task completion; advantage estimation propagates it to earlier invitations and operations. A sampled global STOP receives only its negative decision cost. Forced termination creates no fictitious STOP sample, and outstanding costs are assigned to the last actual transition. With discount one, the sum of decision-level rewards equals Equation~\ref{eq:return}, independently of the number of invitations. Trace decay does not discount the reported task objective, and a rollout boundary does not necessarily terminate an episode.

\textcolor{black}{For task $t$, its final discrete transition $j$ receives $r_j=U_{t+1}-U_t-\lambda_{\mathrm{cost}}c_t$, where $U_t$ is the positive-item log-probability in Equation~\ref{eq:utility} and $c_t$ includes all selection and execution costs for that task. Intermediate transitions receive zero reward, so their logged costs are not charged again. NDCG@20 is an evaluation metric, not the training utility. Generalized Advantage Estimation (GAE) uses discount $\gamma=1.0$ and decay $\lambda_{\mathrm{GAE}}=0.95$. Global STOP, exhaustion of the hard request budget $B=3.0$, or a global execution limit terminates the request: the terminal mask is $d_j=1$ and no value is bootstrapped. A local round limit ends the current task but does not terminate a request that can continue. A sampling truncation within a continuing request uses $d_j=0$ and bootstraps from $V(S_{\mathrm{last}})$. The episode objective is $\Delta U_q-\lambda_{\mathrm{cost}}C_q$, with $\Delta U_q=U_T-U_0$ and $C_q$ the total charged cost.}

\textcolor{black}{\textbf{Author verification:} The previously reported ledger of 1{,}000 rollout episodes, with a maximum reward-reconciliation discrepancy of $<10^{-7}$, must be checked against this log-probability reward and termination convention before it can verify the stated implementation.}

\paragraph{Synchronous execution under a shared budget.}
Individual affordability does not imply joint affordability when multiple members act in one round. Budget reservations must cover the sum of admitted operations and required routing/aggregation overhead. A deterministic reservation procedure may serialize admission while all content observations remain fixed at the round-start snapshot. Its admitted choices and resulting legal masks must be retained for PPO likelihood recomputation. \textcolor{black}{At the start of round $r$, active members propose prospective operations with upper-bound cost allocations (e.g., maximum generation length capped at 128 tokens for textual reasoning; fixed constant cost for deterministic retriever lookups). Operations are admitted sequentially in ascending order of estimated cost until the round budget reservation is satisfied. Variable-length LLM outputs are capped at generation limits; any unused allocation is credited back to the remaining budget upon step completion. If the remaining budget cannot accommodate any nonterminal operation, the request terminates without a sampled STOP action. No extra STOP cost is added; outstanding costs remain assigned to the last actual transition. Identical budget reservation logic and caps are enforced across all matched multi-agent and single-controller baselines.}
